# Supplementary material for: Discovering General-Purpose Active Learning Strategies
Source: arXiv:1810.04114 source file (2019-04-02)
Supplement: Supplementary file 1 [file exp-appendix.tex]

\begin{table*}[t]  
  \centering
  \hspace*{-0.6cm}
  \begin{tabular}{l|r|rrrrrrrrr}
    \toprule
    {\bf Scenario} & test & \multicolumn{9}{c}{leave-one-out} \\
    %\midrule
    {\bf Dataset} & adult & austr & breast & diabet & flare & germ & heart & mush & wave & wdbc \\ 
	\midrule
    \random{} & $\mathit{50.78}$ & $25.31$ & $25.65$ & $30.33$ & $15.57$ & $44.83$ & $20.80$ & $42.81$ & $45.28$ & $19.36$ \\
    \uncertainty{} & \underline{$41.83$} & \bm{$13.53$} & $27.07$ & $\mathit{27.84}$ & $15.50$ & \underline{$37.1$} & \bm{$15.60$} & \bm{$15.6$} & \underline{$23.83$} & \bm{$7.25$} \\
	\QUIRE{} & $58.33$ & $30.02$ & $33.33$ & $37.12$ & \bm{$9.02$} & $57.58$ & $20.30$ & $42.9$ & $\mathit{36.49}$ & $15.45$ \\	
	\ALBE{} & $55.66$ & $29.79$ & $31.84$ & $33.62$ & \underline{$10.91$} & $50.71$ & $21.02$ & $39.12$ & $41.23$ & $16.16$ \\
    \LALindep{} & $59.39$ & $\mathit{20.88}$ & \underline{$20.85$} & \bm{$26.63$} & $15.31$ & $44.14$ & $\mathit{18.16}$ & $\mathit{24.15}$ & $39.13$ & $\mathit{11.22}$ \\
    \vspace{2mm}    
    \LALiter{} & $63.29$ & $\mathit{20.24}$ & \underline{$21.79$} & $28.03$ & $14.84$ & $\mathit{40.38}$ & $19.90$ & $25.2$ & $36.97$ & $\mathit{10.39}$ \\    
	%\midrule
    \RLAL{} & \bm{$37.86$} & \bm{$14.15$} & \bm{$18.79$} & \bm{$26.77$} & $\mathit{14.67}$ & \bm{$32.16$} & \bm{$15.06$} & \underline{$21.94$} & \bm{$20.91$} & \bm{$7.09$} \\
	\RLALnotransf{} & --- & $\color{gray}15.01$ & $\color{gray}16.14$ & $\color{gray}24.40$ & --- & $\color{gray}23.26$ & $\color{gray}14.65$ & $\color{gray}16.47$ & $\color{gray}18.06$ & $\color{gray}7.14$ \\    
    %\midrule
    \bottomrule
    %on adult & --- & $38.80$ & $37.72$ & $36.74$ & $33.95$ & $34.58$ & $38.76$ & $37.46$ & $41.84$ & $37.85$ \\ 
    %\bottomrule
  \end{tabular}
  
  \caption{Average number of annotations to reach a predefined quality level. Leave-one-out experiment and test experiment.}
\label{tab:expUCI}
\end{table*}
